# Supplementary material for: Feasible contact tracing
Source: arXiv:2312.05718 source file (2023-12-10)
Supplement: Supplementary file 1 [file appendix_regret.tex]

\clearpage
\section{Empirical regret}
\textcolor{red}{Not sure if these tables are useful}

In this section, we calculate the regret of each sampler compared to an optimal sampler. The optimal sampler has knowledge of every arm's mean reward. Therefore, it pulls the arm with the largest mean reward among all available arms. We divide the total playing time into four quarters and calculate the regret for each quarter. Some of these regrets may be negative because of the finite sample size.

\subsection{Empirical regret for real data}
\label{section:regret-tables-real-data}

First, we present tables summarizing regret for real data.

\begin{table}[tbh]
    \centering
    \begin{tabular}{c|c|c|c|c}
    Algorithm & Quarter 1 & Quarter 2 & Quarter 3 & Quarter 4 \\
    \hline
    \hline 
	 Pilot Sampling &  325.86 & 240.35 & 116.38 & 34.53 \\ 
	 Adaptive Greedy &  422.85 & 454.94 & 212.9 & 51.76 \\ 
	 Thompson &  362.21 & 287.77 & 118.3 & 33.62 \\ 
	 Naive &  678.51 & 851.13 & 532.32 & 158.51 \\ 

    \end{tabular}
    \caption{Punjab, India}
 \label{tab:punjab-regret}
\end{table}

\begin{table}[tbh]
    \centering
    \begin{tabular}{c|c|c|c|c}
    Algorithm & Quarter 1 & Quarter 2 & Quarter 3 & Quarter 4 \\
    \hline
    \hline 
	 Pilot Sampling &  12648.16 & 9515.94 & 4466.83 & 1111.57 \\ 
	 Adaptive Greedy &  14127.72 & 12819.46 & 7206.35 & 2158.74 \\ 
	 Thompson &  13370.91 & 10362.61 & 4651.02 & 1146.51 \\ 
	 Naive &  15033.53 & 14335.22 & 8596.7 & 2860.44 \\ 

    \end{tabular}
    \caption{Punjab, Pakistan.}
 \label{tab:pakistan-regret}
\end{table}

\begin{table}[tbh]
    \centering
    \begin{tabular}{c|c|c|c|c}
    Algorithm & Quarter 1 & Quarter 2 & Quarter 3 & Quarter 4 \\
    \hline
    \hline 
	 Pilot Sampling &  8602.59 & -3156.42 & -7793.13 & -11096.5 \\ 
	 Adaptive Greedy &  3884.72 & -9674.45 & -9535.21 & -11315.14 \\ 
	 Thompson &  6966.14 & -3286.04 & -7646.75 & -11089.58 \\ 
	 Naive &  12323.15 & 6834.95 & 681.94 & -7910.65 \\ 

    \end{tabular}
    \caption{Southern India.}
 \label{tab:south-regret}
\end{table}

\clearpage
\subsection{Empirical regret for synthetic data}
\label{section:regret-tables}

In this section, we repeat the same exercise as in Appendix \ref{section:regret-tables-real-data} but for the synthetic data.

\begin{table}[tbh]
    \centering
    \begin{tabular}{c|c|c|c|c}
    Algorithm & Quarter 1 & Quarter 2 & Quarter 3 & Quarter 4 \\
    \hline
    \hline 
	 Pilot Sampling &  833.09 & 122.32 & 10.7 & 1.92 \\ 
	 Pilot Sampling (lifetime) &  823.5 & 119.81 & 10.65 & 1.81 \\ 
	 Adaptive Greedy &  628.94 & 660.13 & 188.68 & 21.59 \\ 
	 Adaptive Greedy (lifetime) &  635.22 & 669.9 & 200.27 & 24.54 \\ 
	 Thompson &  214.51 & 92.36 & 11.41 & 2.05 \\ 
	 Naive &  3356.71 & 4633.79 & 2920.38 & 1017.18 \\ 

    \end{tabular}
    \caption{Without branching with Poisson(500) and Beta(0.09, 0.6)}
 \label{tab:nobr-500-009-06}
\end{table}

\begin{table}[tbh]
    \centering
    \begin{tabular}{c|c|c|c|c}
    Algorithm & Quarter 1 & Quarter 2 & Quarter 3 & Quarter 4 \\
    \hline
    \hline 
	 Pilot Sampling &  512.47 & 1601.32 & 2552.81 & 1308.8 \\ 
	 Pilot Sampling (lifetime) &  495.88 & 1570.48 & 2564.04 & 1389.24 \\ 
	 Adaptive Greedy &  26.15 & 90.58 & 156.56 & 254.61 \\ 
	 Adaptive Greedy (lifetime) &  25.38 & 88.67 & 153.92 & 260.06 \\ 
	 Thompson &  35.7 & 45.2 & 67.06 & 64.35 \\ 
	 Naive &  914.73 & 2697.41 & 4366.11 & 3465.67 \\ 

    \end{tabular}
    \caption{Without branching with Poisson(500) and Beta(0.6, 0.09)}
 \label{tab:nobr-500-06-009}
\end{table}

\begin{table}[tbh]
    \centering
    \begin{tabular}{c|c|c|c|c}
    Algorithm & Quarter 1 & Quarter 2 & Quarter 3 & Quarter 4 \\
    \hline
    \hline 
	 Pilot Sampling &  1784.3 & 2965.83 & 1771.36 & 390.86 \\ 
	 Pilot Sampling (lifetime) &  1797.04 & 2928.56 & 1737.63 & 381.16 \\ 
	 Adaptive Greedy &  375.1 & 1042.37 & 1237.64 & 599.41 \\ 
	 Adaptive Greedy (lifetime) &  376.07 & 1058.53 & 1262.49 & 617.28 \\ 
	 Thompson &  274.55 & 369.09 & 248.16 & 77.2 \\ 
	 Naive &  2435.57 & 4875.46 & 4846.14 & 2270.74 \\ 

    \end{tabular}
    \caption{Without branching with Poisson(500) and Beta(1, 1)}
 \label{tab:nobr-500-1-1}
\end{table}

\begin{table}[tbh]
    \centering
    \begin{tabular}{c|c|c|c|c}
    Algorithm & Quarter 1 & Quarter 2 & Quarter 3 & Quarter 4 \\
    \hline
    \hline 
	 Pilot Sampling &  1290.08 & 1486.13 & 862.23 & 170.67 \\ 
	 Pilot Sampling (lifetime) &  1267.14 & 1445.81 & 817.35 & 159.45 \\ 
	 Adaptive Greedy &  625.34 & 1274.48 & 1284.96 & 548.3 \\ 
	 Adaptive Greedy (lifetime) &  634.32 & 1283.08 & 1301.43 & 551.96 \\ 
	 Thompson &  323.28 & 356.58 & 214.24 & 55.96 \\ 
	 Naive &  2001.82 & 3547.94 & 3190.01 & 1402.13 \\ 

    \end{tabular}
    \caption{Without branching with Poisson(500) and Beta(1, 3)}
 \label{tab:nobr-500-1-3}
\end{table}

\begin{table}[tb]
    \centering
    \begin{tabular}{c|c|c|c|c}
    Algorithm & Quarter 1 & Quarter 2 & Quarter 3 & Quarter 4 \\
    \hline
    \hline 
	 Pilot Sampling &  1167.96 & 2702.2 & 2773.33 & 1180.7 \\ 
	 Pilot Sampling (lifetime) &  1155.01 & 2683.15 & 2770.07 & 1221.74 \\ 
	 Adaptive Greedy &  150.15 & 344.28 & 479.34 & 425.72 \\ 
	 Adaptive Greedy (lifetime) &  151.99 & 347.05 & 489.3 & 440.23 \\ 
	 Thompson &  175.52 & 299.87 & 258.57 & 115.11 \\ 
	 Naive &  1309.04 & 3141.08 & 3571.5 & 2179.31 \\ 

    \end{tabular}
    \caption{Without branching with Poisson(500) and Beta(3, 1)}
 \label{tab:nobr-500-3-1}
\end{table}

\begin{table}[tb]
    \centering
    \begin{tabular}{c|c|c|c|c}
    Algorithm & Quarter 1 & Quarter 2 & Quarter 3 & Quarter 4 \\
    \hline
    \hline 
	 Pilot Sampling &  753.93 & 1583.95 & 1425.33 & 628.64 \\ 
	 Pilot Sampling (lifetime) &  779.08 & 1647.12 & 1478.66 & 627.81 \\ 
	 Adaptive Greedy &  383.9 & 693.82 & 613.05 & 333.53 \\ 
	 Adaptive Greedy (lifetime) &  379.64 & 699.67 & 629.09 & 350.81 \\ 
	 Thompson &  373.13 & 485.84 & 347.37 & 148.38 \\ 
	 Naive &  848.79 & 1876.56 & 1877.3 & 935.11 \\ 

    \end{tabular}
    \caption{Without branching with Poisson(500) and Beta(10, 10)}
 \label{tab:nobr-500-10-10}
\end{table}

\begin{table}[tb]
    \centering
    \begin{tabular}{c|c|c|c|c}
    Algorithm & Quarter 1 & Quarter 2 & Quarter 3 & Quarter 4 \\
    \hline
    \hline 
	 Pilot Sampling &  -128.96 & -164.14 & -23.39 & 0.01 \\ 
	 Pilot Sampling (lifetime) &  -158.22 & -157.03 & -14.95 & 0.09 \\ 
	 Adaptive Greedy &  55.86 & 145.98 & 201.08 & 86.56 \\ 
	 Adaptive Greedy (lifetime) &  38.47 & 81.8 & 122.78 & 49.08 \\ 
	 Thompson &  36.54 & 48.5 & 38.37 & 4.05 \\ 
	 Naive &  -16.99 & -47.99 & -10.05 & 16.07 \\ 

    \end{tabular}
    \caption{Without branching with Pareto(1, 0.6) and Beta(0.09, 0.6)}
 \label{tab:nobr-heavytail-009-06}
\end{table}

\begin{table}[tb]
    \centering
    \begin{tabular}{c|c|c|c|c}
    Algorithm & Quarter 1 & Quarter 2 & Quarter 3 & Quarter 4 \\
    \hline
    \hline 
	 Pilot Sampling &  3.63 & 160.35 & 215.93 & -68.61 \\ 
	 Pilot Sampling (lifetime) &  -4.47 & 197.79 & 221.18 & 64.79 \\ 
	 Adaptive Greedy &  21.18 & 33.97 & 37.18 & 0.49 \\ 
	 Adaptive Greedy (lifetime) &  17.64 & 51.95 & 61.78 & 7.95 \\ 
	 Thompson &  15.51 & 20.48 & 11.52 & 0.31 \\ 
	 Naive &  2.82 & 245.46 & 320.54 & 46.8 \\ 

    \end{tabular}
    \caption{Without branching with Pareto(1, 0.6) and Beta(0.6, 0.09)}
 \label{tab:nobr-heavytail-06-009}
\end{table}

\begin{table}[tb]
    \centering
    \begin{tabular}{c|c|c|c|c}
    Algorithm & Quarter 1 & Quarter 2 & Quarter 3 & Quarter 4 \\
    \hline
    \hline 
	 Pilot Sampling &  -19.64 & -273.68 & -203.61 & -5.4 \\ 
	 Pilot Sampling (lifetime) &  -85.76 & -325.92 & -104.37 & 19.85 \\ 
	 Adaptive Greedy &  79.19 & 141.44 & 275.41 & 230.55 \\ 
	 Adaptive Greedy (lifetime) &  43.29 & 74.39 & 127.29 & 119.67 \\ 
	 Thompson &  80.36 & 61.81 & 69.35 & 35.72 \\ 
	 Naive &  59.04 & -105.3 & -87.02 & 76.73 \\ 

    \end{tabular}
    \caption{Without branching with Pareto(1, 0.6) and Beta(1, 1)}
 \label{tab:nobr-heavytail-1-1}
\end{table}

\begin{table}[tb]
    \centering
    \begin{tabular}{c|c|c|c|c}
    Algorithm & Quarter 1 & Quarter 2 & Quarter 3 & Quarter 4 \\
    \hline
    \hline 
	 Pilot Sampling &  -13.85 & -266.41 & -174.41 & 8.34 \\ 
	 Pilot Sampling (lifetime) &  -96.92 & -346.5 & -33.01 & 42.72 \\ 
	 Adaptive Greedy &  79.15 & 140.2 & 273.64 & 237.81 \\ 
	 Adaptive Greedy (lifetime) &  43.24 & 73.94 & 126.3 & 123.33 \\ 
	 Thompson &  80.53 & 61.7 & 69.26 & 37.23 \\ 
	 Naive &  59.32 & -103.83 & -90.14 & 77.7 \\ 

    \end{tabular}
    \caption{Without branching with Pareto(1, 0.6) and Beta(1, 3)}
 \label{tab:nobr-heavytail-1-3}
\end{table}

\begin{table}[tb]
    \centering
    \begin{tabular}{c|c|c|c|c}
    Algorithm & Quarter 1 & Quarter 2 & Quarter 3 & Quarter 4 \\
    \hline
    \hline 
	 Pilot Sampling &  53.65 & 31.99 & -69.63 & -7.33 \\ 
	 Pilot Sampling (lifetime) &  -3.9 & -52.66 & 127.9 & 57.75 \\ 
	 Adaptive Greedy &  46.51 & 72.48 & 98.7 & 101.13 \\ 
	 Adaptive Greedy (lifetime) &  22.88 & 46.26 & 48.14 & 50.7 \\ 
	 Thompson &  53.93 & 69.4 & 76.81 & 67.2 \\ 
	 Naive &  62.55 & 58.17 & -34.16 & 29.83 \\ 

    \end{tabular}
    \caption{Without branching with Pareto(1, 0.6) and Beta(3, 1)}
 \label{tab:nobr-heavytail-3-1}
\end{table}

\begin{table}[tb]
    \centering
    \begin{tabular}{c|c|c|c|c}
    Algorithm & Quarter 1 & Quarter 2 & Quarter 3 & Quarter 4 \\
    \hline
    \hline 
	 Pilot Sampling &  -28.54 & -268.66 & -274.13 & -69.5 \\ 
	 Pilot Sampling (lifetime) &  -106.25 & -344.93 & -105.49 & -5.31 \\ 
	 Adaptive Greedy &  45.21 & 44.5 & 73.85 & 65.63 \\ 
	 Adaptive Greedy (lifetime) &  45.59 & 53.31 & 58.66 & 44.98 \\ 
	 Thompson &  48.58 & 34.28 & 38.12 & 24.98 \\ 
	 Naive &  -30.36 & -270.98 & -253.16 & -35.7 \\ 

    \end{tabular}
    \caption{Without branching with Pareto(1, 0.6) and Beta(10, 10)}
 \label{tab:nobr-heavytail-10-10}
\end{table}

\begin{table}[tb]
    \centering
    \begin{tabular}{c|c|c|c|c}
    Algorithm & Quarter 1 & Quarter 2 & Quarter 3 & Quarter 4 \\
    \hline
    \hline 
	 Pilot Sampling &  25.08 & 46.95 & 7.87 & 1.06 \\ 
	 Pilot Sampling (lifetime) &  24.1 & 44.27 & 8.1 & 1.09 \\ 
	 Adaptive Greedy &  20.38 & 39.06 & 10.91 & 1.55 \\ 
	 Adaptive Greedy (lifetime) &  19.78 & 38.66 & 10.12 & 1.8 \\ 
	 Thompson &  27.63 & 32.01 & 7.53 & 1.02 \\ 
	 Naive &  31.15 & 84.45 & 52.49 & 17.28 \\ 

    \end{tabular}
    \caption{Without branching with Poisson(10) and Beta(0.09, 0.6)}
 \label{tab:nobr-10-009-06}
\end{table}

\begin{table}[tb]
    \centering
    \begin{tabular}{c|c|c|c|c}
    Algorithm & Quarter 1 & Quarter 2 & Quarter 3 & Quarter 4 \\
    \hline
    \hline 
	 Pilot Sampling &  3.51 & 22.45 & 43.33 & 35.68 \\ 
	 Pilot Sampling (lifetime) &  3.72 & 22.15 & 42.44 & 35.58 \\ 
	 Adaptive Greedy &  2.12 & 16.27 & 36.2 & 35.71 \\ 
	 Adaptive Greedy (lifetime) &  2.44 & 16.76 & 35.6 & 33.25 \\ 
	 Thompson &  4.04 & 11.37 & 18.72 & 14.82 \\ 
	 Naive &  5.26 & 31.9 & 62.75 & 61.92 \\ 

    \end{tabular}
    \caption{Without branching with Poisson(10) and Beta(0.6, 0.09)}
 \label{tab:nobr-10-06-009}
\end{table}

\begin{table}[tb]
    \centering
    \begin{tabular}{c|c|c|c|c}
    Algorithm & Quarter 1 & Quarter 2 & Quarter 3 & Quarter 4 \\
    \hline
    \hline 
	 Pilot Sampling &  15.29 & 70.87 & 71.51 & 27.43 \\ 
	 Pilot Sampling (lifetime) &  16.02 & 72.91 & 70.36 & 26.94 \\ 
	 Adaptive Greedy &  13.94 & 61.96 & 62.25 & 31.96 \\ 
	 Adaptive Greedy (lifetime) &  13.11 & 57.3 & 56.74 & 29.96 \\ 
	 Thompson &  23.48 & 56.66 & 52.23 & 27.31 \\ 
	 Naive &  18.12 & 89.29 & 105.05 & 59.33 \\ 

    \end{tabular}
    \caption{Without branching with Poisson(10) and Beta(1, 1)}
 \label{tab:nobr-10-1-1}
\end{table}

\begin{table}[tb]
    \centering
    \begin{tabular}{c|c|c|c|c}
    Algorithm & Quarter 1 & Quarter 2 & Quarter 3 & Quarter 4 \\
    \hline
    \hline 
	 Pilot Sampling &  18.71 & 67.94 & 52.01 & 13.5 \\ 
	 Pilot Sampling (lifetime) &  19.46 & 69.69 & 51.79 & 13.44 \\ 
	 Adaptive Greedy &  16.84 & 57.71 & 50.83 & 17.89 \\ 
	 Adaptive Greedy (lifetime) &  16.42 & 57.85 & 50.17 & 19.15 \\ 
	 Thompson &  22.9 & 57.79 & 46.43 & 14.63 \\ 
	 Naive &  21.2 & 85.3 & 85.64 & 37.04 \\ 

    \end{tabular}
    \caption{Without branching with Poisson(10) and Beta(1, 3)}
 \label{tab:nobr-10-1-3}
\end{table}

\begin{table}[tb]
    \centering
    \begin{tabular}{c|c|c|c|c}
    Algorithm & Quarter 1 & Quarter 2 & Quarter 3 & Quarter 4 \\
    \hline
    \hline 
	 Pilot Sampling &  12.05 & 63.81 & 76.6 & 35.24 \\ 
	 Pilot Sampling (lifetime) &  11.1 & 61.41 & 76.75 & 34.58 \\ 
	 Adaptive Greedy &  9.48 & 51.93 & 63.4 & 32.2 \\ 
	 Adaptive Greedy (lifetime) &  9.4 & 50.58 & 59.92 & 29.2 \\ 
	 Thompson &  18.12 & 46.7 & 47.32 & 25.46 \\ 
	 Naive &  13.97 & 74.75 & 96.06 & 55.13 \\ 

    \end{tabular}
    \caption{Without branching with Poisson(10) and Beta(3, 1)}
 \label{tab:nobr-10-3-1}
\end{table}

\begin{table}[tb]
    \centering
    \begin{tabular}{c|c|c|c|c}
    Algorithm & Quarter 1 & Quarter 2 & Quarter 3 & Quarter 4 \\
    \hline
    \hline 
	 Pilot Sampling &  14.04 & 55.25 & 57.19 & 28.94 \\ 
	 Pilot Sampling (lifetime) &  14.13 & 54.14 & 57.17 & 29.09 \\ 
	 Adaptive Greedy &  13.76 & 51.55 & 54.4 & 29.35 \\ 
	 Adaptive Greedy (lifetime) &  13.79 & 51.1 & 53.04 & 28.72 \\ 
	 Thompson &  17.73 & 52.11 & 54.1 & 29.47 \\ 
	 Naive &  14.37 & 56.72 & 61.15 & 31.9 \\ 

    \end{tabular}
    \caption{Without branching with Poisson(10) and Beta(10, 10)}
 \label{tab:nobr-10-10-10}
\end{table} 

% \subsection{Branching with Poisson(500)}

\begin{table}[tbh]
    \centering
    \begin{tabular}{c|c|c|c|c}
    Algorithm & Quarter 1 & Quarter 2 & Quarter 3 & Quarter 4 \\
    \hline
    \hline 
	 Pilot Sampling &  143.28 & 123.01 & 10.38 & 1.89 \\ 
	 Pilot Sampling (lifetime) &  180.63 & 131.19 & 10.56 & 1.96 \\ 
	 Adaptive Greedy &  1054.27 & 1932.32 & 252.16 & 24.61 \\ 
	 Adaptive Greedy (lifetime) &  1027.24 & 2067.71 & 309.17 & 26.26 \\ 
	 Thompson &  184.61 & 148.29 & 11.27 & 1.93 \\ 
	 Naive &  2537.17 & 4705.96 & 2970.57 & 1023.99 \\ 

    \end{tabular}
    \caption{Branching with Poisson(500) and Beta(0.09, 0.6).}
    \label{tab:br-dense-009-06}
\end{table} 

\begin{table}[tbh]
    \centering
    \begin{tabular}{c|c|c|c|c}
    Algorithm & Quarter 1 & Quarter 2 & Quarter 3 & Quarter 4 \\
    \hline
    \hline 
	 Pilot Sampling &  468.7 & 1542.45 & 2568.94 & 1388.42 \\ 
	 Pilot Sampling (lifetime) &  478.79 & 1536.55 & 2516.09 & 1343.77 \\ 
	 Adaptive Greedy &  27.3 & 90.18 & 155.31 & 255.06 \\ 
	 Adaptive Greedy (lifetime) &  29.36 & 92.62 & 154.58 & 259.71 \\ 
	 Thompson &  28.71 & 45.2 & 68.15 & 64.14 \\ 
	 Naive &  896.13 & 2594.67 & 4292.87 & 3370.12 \\ 

    \end{tabular}
    \caption{Branching with Poisson(500) and Beta(0.6, 0.09).}
    \label{tab:br-dense-06-009}
\end{table}

\begin{table}[tbh]
    \centering
    \begin{tabular}{c|c|c|c|c}
    Algorithm & Quarter 1 & Quarter 2 & Quarter 3 & Quarter 4 \\
    \hline
    \hline 
	 Pilot Sampling &  625.18 & -114.48 & -28.86 & -295.55 \\ 
	 Pilot Sampling (lifetime) &  593.16 & -135.97 & -144.26 & -286.3 \\ 
	 Adaptive Greedy &  -0.1 & -715.08 & -231.37 & -211.65 \\ 
	 Adaptive Greedy (lifetime) &  -17.62 & -760.61 & -23.1 & 255.1 \\ 
	 Thompson &  9.23 & 44.26 & 306.21 & 145.56 \\ 
	 Naive &  1552.86 & 1537.45 & 1889.5 & 1043.64 \\ 

    \end{tabular}
    \caption{Branching with Poisson(500) and Beta(1, 1).}
    \label{tab:br-dense-1-1}
\end{table} 

\begin{table}[tbh]
    \centering
    \begin{tabular}{c|c|c|c|c}
    Algorithm & Quarter 1 & Quarter 2 & Quarter 3 & Quarter 4 \\
    \hline
    \hline 
	 Pilot Sampling &  75.55 & 182.54 & 283.76 & -122.48 \\ 
	 Pilot Sampling (lifetime) &  17.9 & 143.54 & 328.32 & -90.72 \\ 
	 Adaptive Greedy &  -119.63 & 618.67 & 667.3 & 4.5 \\ 
	 Adaptive Greedy (lifetime) &  -43.79 & 882.89 & 1237.5 & 386.18 \\ 
	 Thompson &  -63.1 & 276.39 & 106.33 & 22.53 \\ 
	 Naive &  588.72 & 2008.69 & 2251.82 & 863.52 \\ 

    \end{tabular}
    \caption{Branching with Poisson(500) and Beta(1, 3).}
    \label{tab:br-dense-1-3}
\end{table} 

\begin{table}[tbh]
    \centering
    \begin{tabular}{c|c|c|c|c}
    Algorithm & Quarter 1 & Quarter 2 & Quarter 3 & Quarter 4 \\
    \hline
    \hline 
	 Pilot Sampling &  1113.72 & 2732.87 & 2854.9 & 1255.62 \\ 
	 Pilot Sampling (lifetime) &  1094.71 & 2674.83 & 2790.82 & 1245.07 \\ 
	 Adaptive Greedy &  156.14 & 346.51 & 482.99 & 420.19 \\ 
	 Adaptive Greedy (lifetime) &  149.35 & 350.54 & 488.13 & 438.8 \\ 
	 Thompson &  173.72 & 301.54 & 257.87 & 115.38 \\ 
	 Naive &  1215.57 & 3075.76 & 3544.94 & 2099.22 \\ 

    \end{tabular}
    \caption{Branching with Poisson(500) and Beta(3, 1).}
    \label{tab:br-dense-3-1}
\end{table}

% \begin{table}[tbh]
%     \centering
%     \begin{tabular}{c|c|c|c|c}
%     Algorithm & Quarter 1 & Quarter 2 & Quarter 3 & Quarter 4 \\
%     \hline
%     \hline 
% 	 Pilot Sampling &  19.16 & -3.07 & 17.66 & 78.27 \\ 
% 	 Pilot Sampling (lifetime) &  16.62 & -27.79 & 33.01 & 94.25 \\ 
% 	 Adaptive Greedy &  -340.54 & -542.01 & -451.21 & -191.79 \\ 
% 	 Adaptive Greedy (lifetime) &  -320.47 & -479.06 & -298.86 & 100.03 \\ 
% 	 Thompson &  -238.38 & -200.82 & -51.42 & 37.03 \\ 
% 	 Naive &  41.6 & 94.08 & 201.97 & 307.15 \\ 

%     \end{tabular}
%     \caption{Branching with Poisson(500) and Beta(10, 3).}
%     \label{tab:br-dense-10-3}
% \end{table} 

% \begin{table}[tbh]
%     \centering
%     \begin{tabular}{c|c|c|c|c}
%     Algorithm & Quarter 1 & Quarter 2 & Quarter 3 & Quarter 4 \\
%     \hline
%     \hline 
% 	 Pilot Sampling &  736.79 & 1299.31 & 1002.77 & 400.57 \\ 
% 	 Pilot Sampling (lifetime) &  719.4 & 1279.18 & 994.1 & 400.18 \\ 
% 	 Adaptive Greedy &  568.84 & 994.44 & 889.44 & 492.1 \\ 
% 	 Adaptive Greedy (lifetime) &  573.36 & 1007.58 & 903.9 & 493.53 \\ 
% 	 Thompson &  361.13 & 390.29 & 286.18 & 99.7 \\ 
% 	 Naive &  955.63 & 1902.89 & 1813.94 & 921.63 \\ 

%     \end{tabular}
%     \caption{Branching with Poisson(500) and Beta(3, 10).}
%     \label{tab:br-dense-3-10}
% \end{table} 

\begin{table}[tbh]
    \centering
    \begin{tabular}{l|c|c|c|c}
    Algorithm & Quarter 1 & Quarter 2 & Quarter 3 & Quarter 4 \\
    \hline
    \hline 
	 Pilot Sampling &  646.24 & 1520.25 & 1423.91 & 628.43 \\ 
	 Pilot Sampling (lifetime) &  641.72 & 1509.34 & 1397.63 & 600.19 \\ 
	 Adaptive Greedy &  358.94 & 685.31 & 610.03 & 328.11 \\ 
	 Adaptive Greedy (lifetime) &  358.19 & 691.23 & 624.01 & 341.21 \\ 
	 Thompson &  336.88 & 475.44 & 342.83 & 145.86 \\ 
	 Naive &  710.1 & 1725.34 & 1770.42 & 885.05 \\ 

    \end{tabular}
    \caption{Branching with Poisson(500) and Beta(10, 10).}
    \label{tab:br-dense-10-10}
\end{table}

% \subsection{Branching with Pareto(1, 0.6)}

\begin{table}[tb]
    \centering
    \begin{tabular}{c|c|c|c|c}
    Algorithm & Quarter 1 & Quarter 2 & Quarter 3 & Quarter 4 \\
    \hline
    \hline 
	 Pilot Sampling &  -242.97 & -144.35 & 5.83 & 0.89 \\ 
	 Pilot Sampling (lifetime) &  -243.62 & -144.31 & 4.88 & 0.58 \\ 
	 Adaptive Greedy &  24.68 & 72.2 & 119.45 & 46.04 \\ 
	 Adaptive Greedy (lifetime) &  9.67 & 42.59 & 87.58 & 30.12 \\ 
	 Thompson &  12.93 & 30.98 & 32.44 & 4.02 \\ 
	 Naive &  -242.41 & -143.75 & 17.86 & 20.14 \\ 

    \end{tabular}
    \caption{Branching with Pareto(1, 0.6) and Beta(0.09, 0.6)}
 \label{tab:br-heavytail-009-06}
\end{table}

\begin{table}[tb]
    \centering
    \begin{tabular}{c|c|c|c|c}
    Algorithm & Quarter 1 & Quarter 2 & Quarter 3 & Quarter 4 \\
    \hline
    \hline 
	 Pilot Sampling &  -7.59 & 51.91 & 113.6 & -26.33 \\ 
	 Pilot Sampling (lifetime) &  -13.24 & 14.25 & 64.05 & 71.11 \\ 
	 Adaptive Greedy &  20.54 & 34.4 & 37.3 & 0.65 \\ 
	 Adaptive Greedy (lifetime) &  47.25 & 51.53 & 65.75 & 12.38 \\ 
	 Thompson &  15.85 & 18.84 & 11.11 & 1.08 \\ 
	 Naive &  -7.35 & 59.99 & 124.58 & 3.63 \\ 

    \end{tabular}
    \caption{Branching with Pareto(1, 0.6) and Beta(0.6, 0.09)}
 \label{tab:br-heavytail-06-009}
\end{table}

\begin{table}[tb]
    \centering
    \begin{tabular}{c|c|c|c|c}
    Algorithm & Quarter 1 & Quarter 2 & Quarter 3 & Quarter 4 \\
    \hline
    \hline 
	 Pilot Sampling &  -247.61 & -452.44 & 96.91 & 27.54 \\ 
	 Pilot Sampling (lifetime) &  -255.26 & -451.9 & 57.4 & 25.4 \\ 
	 Adaptive Greedy &  51.49 & 122.59 & 205.49 & 165.56 \\ 
	 Adaptive Greedy (lifetime) &  15.65 & 50.96 & 108.41 & 99.33 \\ 
	 Thompson &  30.96 & 55.48 & 67.26 & 31.11 \\ 
	 Naive &  -233.95 & -450.71 & 132.26 & 140.5 \\ 

    \end{tabular}
    \caption{Branching with Pareto(1, 0.6) and Beta(1, 1)}
 \label{tab:br-heavytail-1-1}
\end{table}

\begin{table}[tb]
    \centering
    \begin{tabular}{c|c|c|c|c}
    Algorithm & Quarter 1 & Quarter 2 & Quarter 3 & Quarter 4 \\
    \hline
    \hline 
	 Pilot Sampling &  -40.98 & -218.35 & -36.49 & 2.49 \\ 
	 Pilot Sampling (lifetime) &  -58.89 & -181.67 & -7.63 & 8.67 \\ 
	 Adaptive Greedy &  69.2 & 158.02 & 275.76 & 148.13 \\ 
	 Adaptive Greedy (lifetime) &  67.54 & 107.36 & 154.21 & 60.42 \\ 
	 Thompson &  49.84 & 59.09 & 55.9 & 12.95 \\ 
	 Naive &  54.13 & -46.07 & 10.18 & 51.32 \\ 

    \end{tabular}
    \caption{Branching with Pareto(1, 0.6) and Beta(1, 3)}
 \label{tab:br-heavytail-1-3}
\end{table}

\begin{table}[tb]
    \centering
    \begin{tabular}{c|c|c|c|c}
    Algorithm & Quarter 1 & Quarter 2 & Quarter 3 & Quarter 4 \\
    \hline
    \hline 
	 Pilot Sampling &  24.49 & -153.61 & -161.83 & -68.3 \\ 
	 Pilot Sampling (lifetime) &  10.88 & -165.1 & -213.13 & -39.6 \\ 
	 Adaptive Greedy &  37.46 & -61.86 & -68.29 & -14.49 \\ 
	 Adaptive Greedy (lifetime) &  33 & 15.11 & -8.04 & -6.9 \\ 
	 Thompson &  41.53 & -80.98 & -90.82 & -48.3 \\ 
	 Naive &  33.68 & -132.25 & -143 & -70.88 \\ 

    \end{tabular}
    \caption{Branching with Pareto(1, 0.6) and Beta(3, 1)}
 \label{tab:br-heavytail-3-1}
\end{table}

\begin{table}[tb]
    \centering
    \begin{tabular}{c|c|c|c|c}
    Algorithm & Quarter 1 & Quarter 2 & Quarter 3 & Quarter 4 \\
    \hline
    \hline 
	 Pilot Sampling &  -157.38 & -467.24 & -63.42 & 10.13 \\ 
	 Pilot Sampling (lifetime) &  -175.18 & -451.55 & -49.02 & 33.38 \\ 
	 Adaptive Greedy &  26.56 & 20.99 & 41.24 & 40.11 \\ 
	 Adaptive Greedy (lifetime) &  62.06 & 50.41 & 47.33 & 38.65 \\ 
	 Thompson &  23.47 & 17.9 & 25.68 & 21.37 \\ 
	 Naive &  -161.59 & -469.32 & -48.44 & 30.89 \\ 

    \end{tabular}
    \caption{Branching with Pareto(1, 0.6) and Beta(10, 10)}
 \label{tab:br-heavytail-10-10}
\end{table} 

% \subsection{Branching with Poisson(10)}

\begin{table}[tb]
    \centering
    \begin{tabular}{c|c|c|c|c}
    Algorithm & Quarter 1 & Quarter 2 & Quarter 3 & Quarter 4 \\
    \hline
    \hline 
	 Pilot Sampling &  39.26 & 50.28 & 13.55 & 0.97 \\ 
	 Pilot Sampling (lifetime) &  39.03 & 49.72 & 13.32 & 1.16 \\ 
	 Adaptive Greedy &  38.85 & 60.8 & 25.83 & 3.81 \\ 
	 Adaptive Greedy (lifetime) &  38.18 & 58.35 & 21.02 & 2.8 \\ 
	 Thompson &  36.09 & 46.36 & 10.14 & 0.91 \\ 
	 Naive &  52.56 & 90.04 & 56.81 & 20.19 \\ 

    \end{tabular}
    \caption{Branching with Poisson(10) and Beta(0.09, 0.6)}
 \label{tab:br-10-009-06}
\end{table} 
\begin{table}[tb]
    \centering
    \begin{tabular}{c|c|c|c|c}
    Algorithm & Quarter 1 & Quarter 2 & Quarter 3 & Quarter 4 \\
    \hline
    \hline 
	 Pilot Sampling &  9.99 & 30.79 & 46.08 & 27.86 \\ 
	 Pilot Sampling (lifetime) &  9.5 & 30.13 & 44.99 & 27.6 \\ 
	 Adaptive Greedy &  7.44 & 24.9 & 40.79 & 31.64 \\ 
	 Adaptive Greedy (lifetime) &  6.74 & 24.11 & 39.56 & 28.36 \\ 
	 Thompson &  6.5 & 14.73 & 16.77 & 17.09 \\ 
	 Naive &  15.39 & 46.33 & 72.92 & 62.22 \\ 

    \end{tabular}
    \caption{Branching with Poisson(10) and Beta(0.6, 0.09)}
 \label{tab:br-10-06-009}
\end{table} 
\begin{table}[tb]
    \centering
    \begin{tabular}{c|c|c|c|c}
    Algorithm & Quarter 1 & Quarter 2 & Quarter 3 & Quarter 4 \\
    \hline
    \hline 
	 Pilot Sampling &  27.19 & 58 & 50.62 & 26.94 \\ 
	 Pilot Sampling (lifetime) &  28.83 & 61.4 & 51.25 & 26.65 \\ 
	 Adaptive Greedy &  22.48 & 49.81 & 50.95 & 31.62 \\ 
	 Adaptive Greedy (lifetime) &  23.03 & 48.48 & 47.99 & 31.09 \\ 
	 Thompson &  19.44 & 40.57 & 44.95 & 28.38 \\ 
	 Naive &  33.62 & 78.95 & 84.11 & 50.64 \\ 

    \end{tabular}
    \caption{Branching with Poisson(10) and Beta(1, 1)}
 \label{tab:br-10-1-1}
\end{table} 
\begin{table}[tb]
    \centering
    \begin{tabular}{c|c|c|c|c}
    Algorithm & Quarter 1 & Quarter 2 & Quarter 3 & Quarter 4 \\
    \hline
    \hline 
	 Pilot Sampling &  31.87 & 56.94 & 49.11 & 20.48 \\ 
	 Pilot Sampling (lifetime) &  30.94 & 56.48 & 48.77 & 21.02 \\ 
	 Adaptive Greedy &  30.85 & 59.26 & 54.51 & 25.58 \\ 
	 Adaptive Greedy (lifetime) &  30.93 & 57.49 & 54.23 & 27.26 \\ 
	 Thompson &  28.48 & 52.5 & 46.98 & 19.83 \\ 
	 Naive &  39.56 & 80.83 & 79.14 & 40.42 \\ 

    \end{tabular}
    \caption{Branching with Poisson(10) and Beta(1, 3)}
 \label{tab:br-10-1-3}
\end{table} 
\begin{table}[tb]
    \centering
    \begin{tabular}{c|c|c|c|c}
    Algorithm & Quarter 1 & Quarter 2 & Quarter 3 & Quarter 4 \\
    \hline
    \hline 
	 Pilot Sampling &  26.96 & 64.87 & 71.03 & 28.9 \\ 
	 Pilot Sampling (lifetime) &  27.79 & 66.63 & 72.87 & 30.86 \\ 
	 Adaptive Greedy &  22.25 & 54.65 & 63.37 & 30.15 \\ 
	 Adaptive Greedy (lifetime) &  20.91 & 52.82 & 59.12 & 27.36 \\ 
	 Thompson &  20.23 & 41.5 & 45.4 & 22.86 \\ 
	 Naive &  32.29 & 79.83 & 93.21 & 48.93 \\ 

    \end{tabular}
    \caption{Branching with Poisson(10) and Beta(3, 1)}
 \label{tab:br-10-3-1}
\end{table} 
\begin{table}[tb]
    \centering
    \begin{tabular}{c|c|c|c|c}
    Algorithm & Quarter 1 & Quarter 2 & Quarter 3 & Quarter 4 \\
    \hline
    \hline 
	 Pilot Sampling &  16.4 & 36.28 & 52.08 & 33.87 \\ 
	 Pilot Sampling (lifetime) &  15.65 & 33.29 & 48.8 & 33.77 \\ 
	 Adaptive Greedy &  19.31 & 39.26 & 54.86 & 37.7 \\ 
	 Adaptive Greedy (lifetime) &  17.06 & 35.36 & 50.18 & 33.9 \\ 
	 Thompson &  18.97 & 41.55 & 60.47 & 41.09 \\ 
	 Naive &  16.25 & 36.88 & 53.43 & 36.88 \\ 

    \end{tabular}
    \caption{Branching with Poisson(10) and Beta(10, 10)}
 \label{tab:br-10-10-10}
\end{table}
